# Supplementary material for: Crystalline Electric-Field Excitations in Quantum Spin Liquids Candidate $NaYbSe_{2}$
Source: arXiv:2002.04772 source file (2020-02-16)
Supplement: Supplementary file 1 [file supplement.pdf]

# Supplementary Material: Crystalline Electric-Field Excitations in Quantum Spin Liquids Candidate $NaYbSe_2$


Zheng Zhang, Jianshu Li, Weiwei Liu, and Yimeng Wang
*Beijing National Laboratory for Condensed Matter Physics,*
*Institute of Physics, Chinese Academy of Sciences, Beijing 100190, China and*
*Department of Physics, Renmin University of China, Beijing 100872, China*

Xiaoli Ma, Feng Jin, and Jianting Ji
*Beijing National Laboratory for Condensed Matter Physics,*
*Institute of Physics, Chinese Academy of Sciences, Beijing 100190, China*

Guohua Wang, Xiaoqun Wang, and Jie Ma*
*Department of Physics and Astronomy, Shanghai Jiao Tong University, Shanghai 200240, China*

D.T. Adroja
*ISIS Neutron and Muon Facility, SCFT Rutherford Appleton Laboratory,*
*Chilton, Didcot Oxon, OX11 0QX, United Kingdom and*
*Highly Correlated Matter Research Group, Physics Department,*
*University of Johannesburg, Auckland Park 2006, South Africa*

T.G. Perring
*ISIS Neutron and Muon Facility, SCFT Rutherford Appleton Laboratory,*
*Chilton, Didcot Oxon, OX11 0QX, United Kingdom*

Qingming Zhang†
*School of Physical Science and Technology, Lanzhou University, Lanzhou 730000, China and*
*Beijing National Laboratory for Condensed Matter Physics,*
*Institute of Physics, Chinese Academy of Sciences, Beijing 100190, China*



(Dated: February 12, 2020)


We present here:
1. Sample Synthesis Method, X-ray Diffraction(XRD) and Energy Dispesive X-ray(EDX)
2. Theory of Crystalline Electric-Field(CEF) and Inelastic Neutron Scattering(INS)
3. Point Charge Model(PCM)
4. Analysis of Phonon Symmetry and Raman Scattering(RS)


* e-mail:jma3@sjtu.edu.cn
† e-mail:qmzhang@ruc.edu.cn

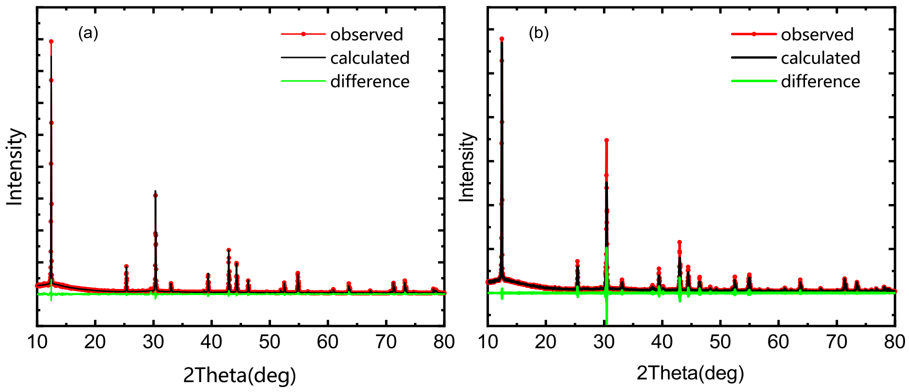


FIG. 1. $NaYbSe_2$ and $NaLuSe_2$ powder diffraction patterns and Rietveld refinements .

# I. SAMPLE SYNTHESIS METHOD, X-RAY DIFFRACTION(XRD) AND ENERGY DISPESIVE X-RAY(EDX)

## A. Single crystal

The high quality $NaReSe_2$(Re=Yb or Lu) single crystals were grown using a NaCl-flux method [1, 2]. The chemical reaction equation is expressed as follows:

$$NaCl + Re + 2Se \longrightarrow NaReSe_2 \tag{1}$$

NaCl, Re and Se powders are mixed in an argon-filled glove box (mixing mass ration: NaCl:Re:Se=10:2:2). Since the saturated vapor pressure of selenium rises rapidly at more than 1000°C, we designed quartz tubes that can withstand higher vapor pressure. The mixed powder was placed in the special quartz tube and vacuum sealed. The quartz tube was headed up to 1000℃ for 1440 minutes and maintained for 10000 minutes, then slowly cooled down to 750℃ for 9000 minutes and cooled down to 500℃ for 3000 minutes. After the heating and cooling, we can observe $NaReSe_2$ single crystals in NaCl interlayer. After rinsing with deionized water and alcohol, single crystal sizes of 10-20 mm can be obtained.

## B. polycrystalline

The synthesis of polycrystalline $NaYbSe_2$ is relatively simple. The chemical equation of solid phase reaction at high temperature is as follows[3]:

$$Na_2Se + 2Yb + 3Se \longrightarrow 2NaYbSe_2 \tag{2}$$

$Na_2Se$, Yb and Se powders were mixed in an argon-filled glove box. The materials with molar ratio of $Na_2Se$:Yb:Se = 1:2:3 are added to graphite crucible, which is placed in a 3mm wall thickness quart tube and vacuum sealed. The mixed materials are heated up to 900℃ for 1440 minutes and maintains for 4320 minutes, then cooled naturally to room temperature. Finally, we can obtain $NaYbSe_2$ polycrystalline samples.

## C. X-ray Diffraction(XRD)

The polycrystalline samples were confirmed by powder X-ray diffraction(XRD) (Brucker D8 Advance, 40 kV, 40 mA). FIG.1 shows the powder diffraction patterns and Rietveld refinements for $NaYbSe_2$ and $NaLuSe_2$.

The refinements results are shown in the TABLE I.

TABLE I. X-ray diffraction and structural refinement for $NaReSe_2$(Re=Yb,Lu)

| Compound | | $NaYbSe_2$ | $NaLuSe_2$ |
|---|---|---|---|
| Radition | | Cu $K_\alpha$ | Cu $K_\alpha$ |
| Temperature | | 300K | 300K |
| symmetry | | R-3m | R-3m |
| Lattice | a=b | 4.05753Å | 4.0304Å |
| constants | c | 20.7744Å | 20.0644Å |
| Cell volume | V | 296.1973Å$^3$ | 325.9286Å$^3$ |
| Crystal size | L | 1409.8 nm | 46.5nm |
| | G | 3612.0 nm | 56.5nm |
| Residuals | | 0.08207 | 0.09424 |
| | | Atom site | |
| $Na^+$ | x=y | 0 | 0 |
| | z | 0.5 | 0.5 |
| Occupany | | 1 | 1 |
| $Re^{+3}$ (Re=Yb,Lu) | x=y | 0 | 0 |
| | z | 0 | 0 |
| Occupancy | | 1 | 1 |
| $Se^{-2}$ | x=y | 0 | 0 |
| | z | 0.25811 | 0.25723 |
| Occupancy | | 1 | 1 |

TABLE II. Element compositions of $NaYbSe_2$ and $NaLuSe_2$

| | Na | Yb or Lu | Se |
|---|---|---|---|
| (a) | 24.55% | 23.14% | 52.31% |
| (b) | 24.54% | 25.95% | 49.51% |
| (c) | 23.25% | 24.89% | 51.87% |
| (d) | 25.01% | 24.80% | 50.19% |
| (e) | 26.14% | 24.99% | 48.87% |
| (f) | 25.33% | 24.94% | 49.73% |

### D. Energy Dispesive X-ray(EDX)

Single crystal samples and powder sample elements compositions were determined by scanning electron microscope (Nova NanoSEM 450) − Energy dispersive X-ray (EDS Inca X-Max, Oxford Instruments).

For $NaYbSe_2$ and $NaLuSe_2$ powder and single crystal, the elements composition rations were determined by the energy dispersion x-ray spectrum(EDX). The scanning electron microscope photographs of single in ab-plane and elemental proportions were shown in the following FIG. 2 and TABLE II. Accrording to the elemental composition anlysis in the TABLE II, there is amost no atomic vacancy in the $NaYbSe_2$ and $NaLuSe_2$ samples. The high quality powder and single crystal are closely related to the physical and chemical properties of alkali metal elements, rare earth elements and sulfur group elements.

## II. THEORY OF CRYSTALLINE ELECTRIC-FIELD(CEF) AND INELASTIC NEUTRON SCATTERING(INS)

The CEF excitations of $NaYbSe_2$ were measured by inelastic neutron scattering(INS). Accoring to CEF theory of rare earth ions, the CEF parameters, excitation levels and wave functions of $NaYbSe_2$ are obtained by fitting and calculation. The following is the detailed results obtained by our fitting and calculation.

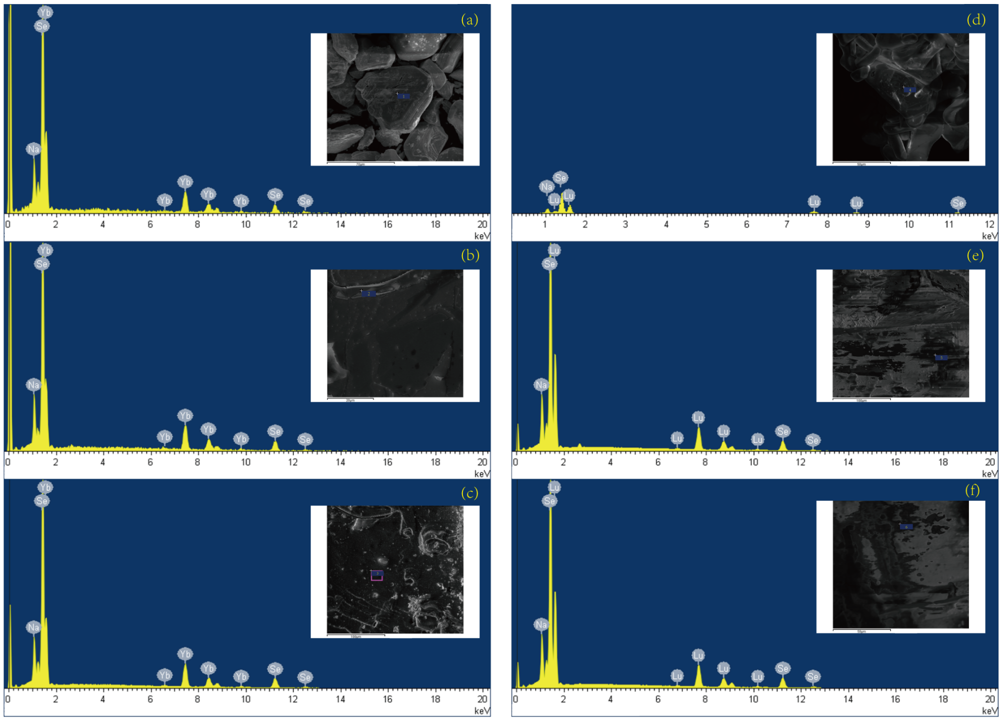


FIG. 2. Electron micrograph and elemental analysis for $NaYbSe_2$ and $NaLuSe_2$. (a) and (d) are powder samples of $NaYbSe_2$ and $NaLuSe_2$ respectively. (b) and (c) are single crystal sample of $NaYbSe_2$. (e) and (f) are single crystal sample for $NaLuSe_2$

### A. Crystalline Electric-Field(CEF) Hamiltonian and differental neutron cross section

Free $Yb^{3+}(4f^{13})$ ion has the orbital angular momentum $L = 3$ and the spin angular momentum $s = 1/2$. $Yb_3^+$ ion has total angular momentum $J = 7/2$ and Lande $g$ factor $g_J = 8/7$ due to the strong spin orbital coupling(SOC) of $4f$ electron.

In the QSLs candidate materials $NaYbSe_2$,$Yb^{3+}$ ions form the octahedral structure of $YbSe_6$ with the surrounding ligand anions.The structure of $YbSe_6$ has point group symmetry of $D_{3d}$ and the $Yb^{3+}$ ion which is influenced by the CEF formed by surrounding Se anions splits into four Kramers doublets. So, the CEF Hamiltonian of $NaYbSe_2$ can be expressed as follows[4–6]

$$H_{CEF} = B_2^0 O_2^0 + B_4^0 O_4^0 + B_4^3 O_4^3 + B_6^0 O_6^0 + B_6^3 O_6^3 + B_6^6 O_6^6 \tag{3}$$

where $B_m^n$ are CEF parameters which are related to the electronic structure of the rare-earth material, and the Stevens operatirs $O_m^n$ are analytic polynomial related to the angular momentum operators $J_+$, $J_-$ and $J_z$. The $O_m^n$ operators are represented as follows[6]

$$O_2^0 = 3J_z^2 - X, \tag{4}$$

$$O_4^0 = 35J_z^4 - (30X - 25)J_z^2 + 3X^2, \tag{5}$$

$$O_4^3 = \frac{1}{4}[(J_+^3 + J_-^3)J_z + J_z(J_+^3 + J_-^3)], \tag{6}$$

$$O_6^0 = 231J_z^6 - (315X - 735)J_z^4 + (105X^2 - 525X + 249)J_z^2 - 5X^3 + 40X^2 - 60X, \tag{7}$$

$$O_6^3 = \frac{1}{4}[(J_+^3 + J_-^3)(11J_z^3 - (3X + 59)J_z) + (11J_z^3 - (3X + 59)J_z)(J_+^3 + J_-^3)], \tag{8}$$

$$O_6^6 = \frac{1}{2}(J_+^6 + J_-^6) \tag{9}$$

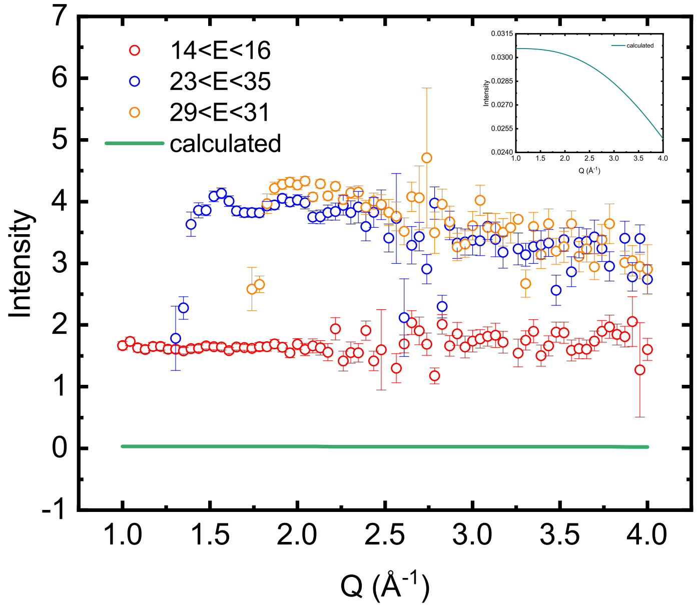


FIG. 3. $NaYbSe_2$ and $NaLuSe_2$ powder diffraction patterns and Rietveld refinements .

TABLE III. $\langle j_0 \rangle$ and $\langle j_2 \rangle$ form factors for $Yb^{+3}$ ion

| index | A | a | B | b | C | c | D |
|---|---|---|---|---|---|---|---|
| $\langle j_0 \rangle$ | 0.0416 | 16.095 | 0.2849 | 7.834 | 0.6971 | 2.672 | -0.0229 |
| $\langle j_2 \rangle$ | 0.1570 | 18.555 | 0.8484 | 6.540 | 0.8880 | 2.037 | 0.0318 |

where $X = J(J+1)$. The eigenstates(Kramers doublet) of the CEF Hamiltonian can be written as the follows

$$|\psi_{k,\pm}\rangle = \sum_{m_J=-7/2}^{7/2} C_{m_J}^{k,\pm} |J = 7/2, m_J\rangle \tag{10}$$

where $C_{m_J}^{k,\pm}$ is the weight cofficient of each eigenstates.

For $NaYbSe_2$, the differental neutron cross section of powder sample for the CEF Kramers double transition $|\psi_{k_i}\rangle$ to $|\psi_{k_f}\rangle$ is given in the dipole approximation by[5, 7, 8]:

$$\frac{d^2\sigma}{d\Omega d\omega} = C\frac{k_f}{k_i}F^2(|\overrightarrow{Q}|)exp\left(\frac{-\hbar\omega_{k_i}}{k_BT}\right) \times \sum_{\alpha=x,y,z} \left|\langle\psi_{k_f}|J_\alpha|\psi_{k_i}\rangle\right|^2 L(\omega_{k_i} - \omega_{k_f} + \omega) \tag{11}$$

where $F\left(\left|\overrightarrow{Q}\right|\right) = \left\langle j_0\left(\left|\overrightarrow{Q}\right|\right)\right\rangle + \frac{2-g_J}{g_J}\left\langle j_2\left(\left|\overrightarrow{Q}\right|\right)\right\rangle$ is the magnetic form factor in the dipole approxmiation.

$$\left\langle j_0\left(\left|\overrightarrow{Q}\right|\right)\right\rangle = A_0 \exp\left(-a_0\left|\overrightarrow{Q}\right|^2\right) + B_0 \exp\left(-b_0\left|\overrightarrow{Q}\right|^2\right) + C_0 \exp\left(-c_0\left|\overrightarrow{Q}\right|^2\right) + D_0, \tag{12}$$

$$\left\langle j_2\left(\left|\overrightarrow{Q}\right|\right)\right\rangle = A_2\left|\overrightarrow{Q}\right|^2 \exp\left(-a_2\left|\overrightarrow{Q}\right|^2\right) + B_2\left|\overrightarrow{Q}\right|^2 \exp\left(-b_2\left|\overrightarrow{Q}\right|^2\right) + C_2\left|\overrightarrow{Q}\right|^2 \exp\left(-c_2\left|\overrightarrow{Q}\right|^2\right) + D_2\left|\overrightarrow{Q}\right|^2 \tag{13}$$

The $A_0, a_0, B_0, b_0, C_0, c_0, D_0$ and $A_2, a_2, B_2, b_2, C_2, c_2, D_2$ are neutron magnetic formfactor coefficients.[9] TABLE III is $\langle j_0 \rangle$ form factors for $Yb^{+3}$ and $\langle j_2 \rangle$ form factors for $Yb^{+3}$.

FIG. 3 shows the momentum transfer $|Q|$ dependences of INS intensities integrated over the energy ranges, $14 < E < 16$ meV, $23 < E < 35$ meV and $29 < E < 31$ meV, respectively. The insert of FIG. 3 calculate the magnetic

TABLE IV. Fitting results of $NaYbSe_2$ CEF at different temperature

| Measurement Temperature | 5K | | 100K | | 150K | | 200K | | 300K | |
|---|---|---|---|---|---|---|---|---|---|---|
| | Exp. | Calc. | Exp. | Calc. | Exp. | Calc. | Exp. | Calc. | Exp. | Calc. |
| $\hbar\omega1$(meV) | 15.75 | 15.79 | 15.85 | 16.56 | 17.25 | 17.76 | 18.04 | 17.94 | 18.65 | 18.75 |
| $\hbar\omega2$(meV) | 24.45 | 24.33 | 24.55 | 24.59 | 25.25 | 25.23 | 26.05 | 26.11 | 27.25 | 27.28 |
| $\hbar\omega2$(meV) | 30.45 | 30.53 | 30.85 | 30.74 | 31.15 | 31.28 | 32.05 | 31.94 | 33.25 | 33.32 |
| $g_{c-axis}$ | 1.05 | | 1.06 | | 0.90 | | 0.90 | | 0.86 | |
| $g_{ab-plane}$ | 2.81 | | 2.89 | | 3.10 | | 2.92 | | 2.69 | |
| $B_2^0$(meV) | -0.1579 | | -0.1571 | | -0.2238 | | -0.1542 | | -0.2082 | |
| $B_4^0$(meV) | 0.0110 | | 0.0110 | | 0.0064 | | 0.0108 | | 0.0117 | |
| $B_4^3$(meV) | -0.0999 | | -0.0994 | | -0.1444 | | -0.1155 | | -0.0687 | |
| $B_6^0$(meV) | 0 | | 0 | | -0.0002 | | 0 | | 0 | |
| $B_6^3$(meV) | -0.0025 | | -0.0025 | | -0.0027 | | -0.0019 | | -0.0031 | |
| $B_6^6$(meV) | 0.0133 | | 0.0135 | | 0.0143 | | 0.0144 | | 0.0152 | |

form factor $F(|Q|)$ based on the dipole approxmiation. The change trend of the calculated results is consistent with the experiment.

The CEF parameters allow us to estimate the $g$ factor using the following formula:

$$g_{ab-plane} = g_J \left|\langle\psi_{0,\pm}\right| m_{J\pm} \left|\psi_{0,\mp}\rangle\right| \tag{14}$$

$$g_{c-axis} = 2g_J \left|\langle\psi_{0,\pm}\right| m_{Jz} \left|\psi_{0,\pm}\rangle\right| \tag{15}$$

where $g_J$ is Lande factor which is 7/2 for $Yb^{3+}$ ion, $\langle\psi_{0,\pm}|$ and $|\psi_{0,\mp}\rangle$ are eigen states, and $m_{J\pm}/m_{Jz}$ are ladder operators.

### B. $NaYbSe_2$ CEF fitting

The CEF fits to the experimental data are performed using Python programs based on Mantid[10, 11]. The calcuation of the CEF energy levels and g factors are performed using MATLAB.

Table 4 and Table 5 are respectively the CEF parameters and wave functions obtained by $NaYbSe_2$ fitting at different temperatures.

### C. $NaLuSe_2$ INS cuts

FIG. 4 is cuts of INS spectrum of $NaLuSe_2$ at different temperatures. The red dotted lines mark the phonon excitation of $NaLuSe_2$.

### D. Comparison charts at different temperatures of $NaYbSe_2$ and $NaLuSe_2$ INS cuts

FIG. 5 is the comparsion chart at 5 different temperatures of $NaYbSe_2$ INS cuts. FIG. 6 is the comparsion chart at 3 different temperatures of $NaLuSe_2$ INS cuts;

## III. POINT CHARGE MODEL(PCM)

The point charge model can be used to calculate the CEF parameters. Under the point charge model approximation, the CEF parameters can be expressed as follows[5, 10–12]:

$$B_l^m = \frac{4\pi}{2l+14}\frac{|e|^2}{4\pi\varepsilon_0}\sum_i \frac{q_i}{r_i^{l+1}} a_0^l < r^l > Z_l^m(\theta_i, \psi_i) \tag{16}$$

TABLE V. Fitted CEF Wavefunctions

| |
|---|
| Fit at 5K |
| $\vert\varphi_{0,\pm}\rangle = +0.8019\,\vert\pm5/2\rangle \pm 0.1368\,\vert\mp1/2\rangle - 0.5693\,\vert\mp7/2\rangle$ |
| $\vert\varphi_{1,\pm}\rangle = -0.1396\,\vert\pm3/2\rangle \pm 0.9902\,\vert\mp3/2\rangle$ |
| $\vert\varphi_{2,\pm}\rangle = -0.4716\,\vert\pm5/2\rangle \pm 0.7307\,\vert\mp1/2\rangle - 0.4887\,\vert\mp7/2\rangle$ |
| $\vert\varphi_{3,\pm}\rangle = -0.3524\,\vert\pm5/2\rangle \mp 0.6665\,\vert\mp1/2\rangle - 0.6565\,\vert\mp7/2\rangle$ |
| Fit at 100K |
| $\vert\varphi_{0,\pm}\rangle = \pm0.5737\,\vert\pm7/2\rangle + 0.1364\,\vert\pm1/2\rangle \mp 0.8065\,\vert\mp5/2\rangle$ |
| $\vert\varphi_{1,\pm}\rangle = +0.0661\,\vert\pm3/2\rangle \mp 0.9978\,\vert\mp3/2\rangle$ |
| $\vert\varphi_{2,\pm}\rangle = -0.4647\,\vert\pm5/2\rangle \pm 0.7453\,\vert\mp1/2\rangle - 0.4761\,\vert\mp7/2\rangle$ |
| $\vert\varphi_{3,\pm}\rangle = -0.3633\,\vert\pm5/2\rangle - 0.6517\,\vert\mp1/2\rangle \mp 0.6656\,\vert\mp7/2\rangle$ |
| Fit at 150K |
| $\vert\varphi_{0,\pm}\rangle = +0.6762\,\vert\pm7/2\rangle \pm 0.2234\,\vert\pm1/2\rangle - 0.7021\,\vert\mp5/2\rangle$ |
| $\vert\varphi_{1,\pm}\rangle = \mp0.0576\,\vert\pm3/2\rangle + 0.9983\,\vert\mp3/2\rangle$ |
| $\vert\varphi_{2,\pm}\rangle = \mp0.5707\,\vert\pm5/2\rangle + 0.7444\,\vert\mp1/2\rangle \mp 0.3466\,\vert\mp7/2\rangle$ |
| $\vert\varphi_{3,\pm}\rangle = -0.6499\,\vert\pm7/2\rangle \pm 0.6290\,\vert\pm1/2\rangle - 0.4258\,\vert\mp5/2\rangle$ |
| Fit at 200K |
| $\vert\varphi_{0,\pm}\rangle = \pm0.5810\,\vert\pm7/2\rangle + 0.1634\,\vert\pm1/2\rangle \mp 0.7973\,\vert\mp5/2\rangle$ |
| $\vert\varphi_{1,\pm}\rangle = -0.3116\,\vert\pm3/2\rangle \pm 0.9502\,\vert\mp3/2\rangle$ |
| $\vert\varphi_{2,\pm}\rangle = \mp0.4550\,\vert\pm5/2\rangle + 0.7949\,\vert\mp1/2\rangle \mp 0.4009\,\vert\mp7/2\rangle$ |
| $\vert\varphi_{3,\pm}\rangle = +0.3963\,\vert\pm5/2\rangle + 0.5841\,\vert\mp1/2\rangle \pm 0.7083\,\vert\mp7/2\rangle$ |
| Fit at 300K |
| $\vert\varphi_{0,\pm}\rangle = \mp0.5785\,\vert\pm7/2\rangle - 0.1498\,\vert\pm5/2\rangle \pm 0.7905\,\vert\mp5/2\rangle$ |
| $\vert\varphi_{1,\pm}\rangle = -0.3116\,\vert\pm3/2\rangle \pm 0.9502\,\vert\mp3/2\rangle$ |
| $\vert\varphi_{2,\pm}\rangle = +0.4361\,\vert\pm5/2\rangle \mp 0.7482\,\vert\mp1/2\rangle + 0.4982\,\vert\mp7/2\rangle$ |
| $\vert\varphi_{3,\pm}\rangle = \mp0.4024\,\vert\pm5/2\rangle - 0.6580\,\vert\mp1/2\rangle \mp 0.6359\,\vert\mp7/2\rangle$ |

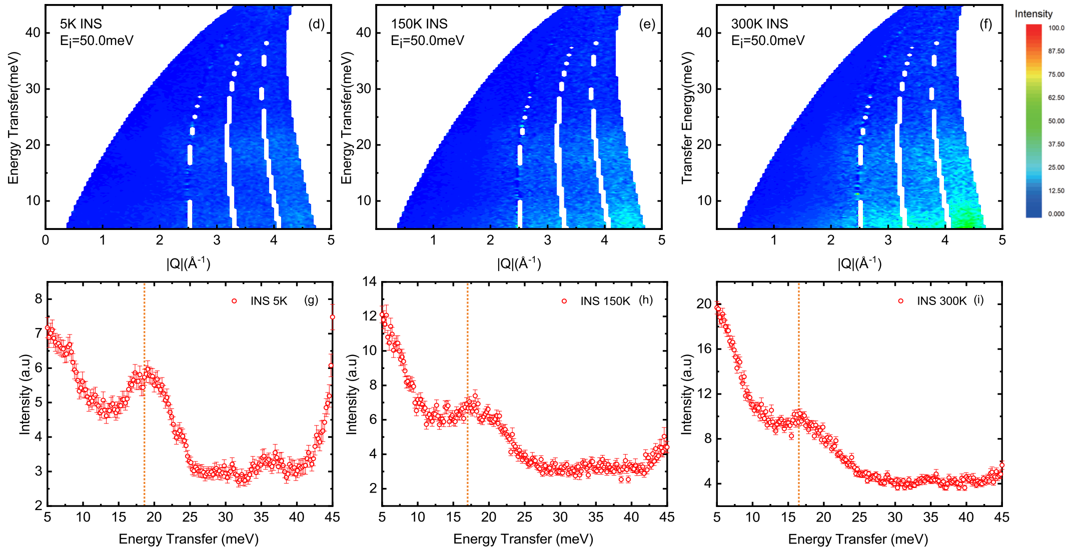


FIG. 4. INS spectrum and cuts of INS spectrum of $NaLuSe_2$ at different temperatures

where $q_i$ is charge, $r_i$, $\theta_i$ and $\phi_i$ are the relative polar coordinates of the $i^{th}$ point chargs from the magnetic ion. $a_0$ is the Bohr radius, $< r^l >$ is the $l^{th}$ order expectation value of the radial wavefunction of the magnetic ion.

We use the point charge model to calculate the CEF parameters of $NaYbO_2$, $NaYbS_2$ and $NaYbSe_2$. The calculation results are shown in the Table 6.

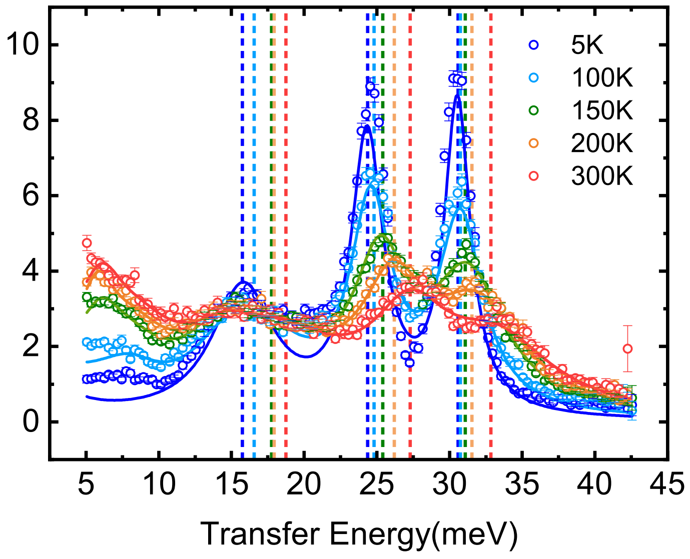


FIG. 5. INS cuts of $NaYbSe_2$ at five temperatures.

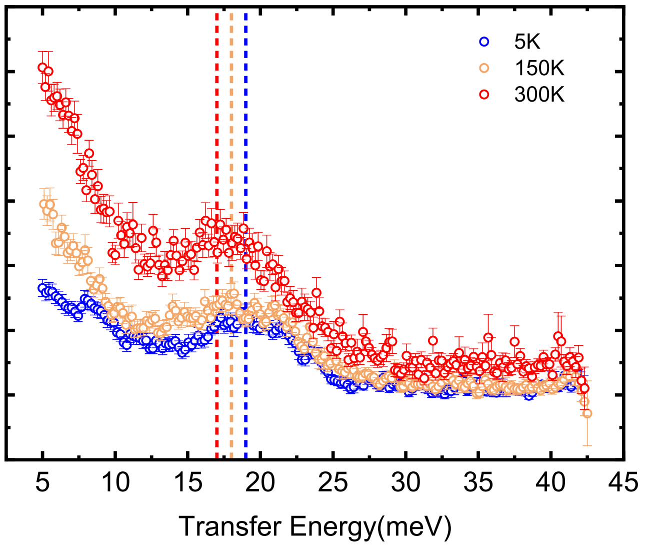


FIG. 6. INS cuts of $NaLuSe_2$ at three temperatures.

## IV. ANALYSIS OF PHONON SYMMETRY AND RAMAN SCATTERING(RS)

The space group of $NaYbSe_2$ and $NaLuSe_2$ are R-3m. The point group of $NaYbSe_2$ and $NaLuSe_2$ are $D_{3d}$. According to the symmetry analysis, two Raman active phonons can be observed in the experiment. The vibration modes of these two phonons are $E_g$ and $A_{1g}$ respectively, where the $E_g$ model is degenerate. The Raman tensor of the two phonon modes are expressed as follows[13, 14]:

TABLE VI. CEF energy levels and CEF parameters of $NaYbO_2$, $NaYbS_2$ and $NaYbSe_2$ based on point charge model

| Sample | $NaYbO_2$ | $NaYbS_2$ | $NaYbSe_2$ |
|---|---|---|---|
| $\hbar\omega_1$(meV) | 39.6886 | 20.19 | 16.52 |
| $\hbar\omega_2$(meV) | 91.1681 | 44.61 | 36.47 |
| $\hbar\omega_3$(meV) | 123.4349 | 60.00 | 49.12 |
| $B_2^0$(meV) | -3.3008 | -1.6118 | -1.3195 |
| $B_4^0$(meV) | 0.0162 | 0.0073 | 0.0060 |
| $B_4^3$(meV) | -0.3292 | -0.1429 | -0.1161 |
| $B_6^0$(meV) | 0 | 1.8795 | 0 |
| $B_6^3$(meV) | 0 | 0 | 0.0003 |
| $B_6^6$(meV) | 0 | 0 | 0 |

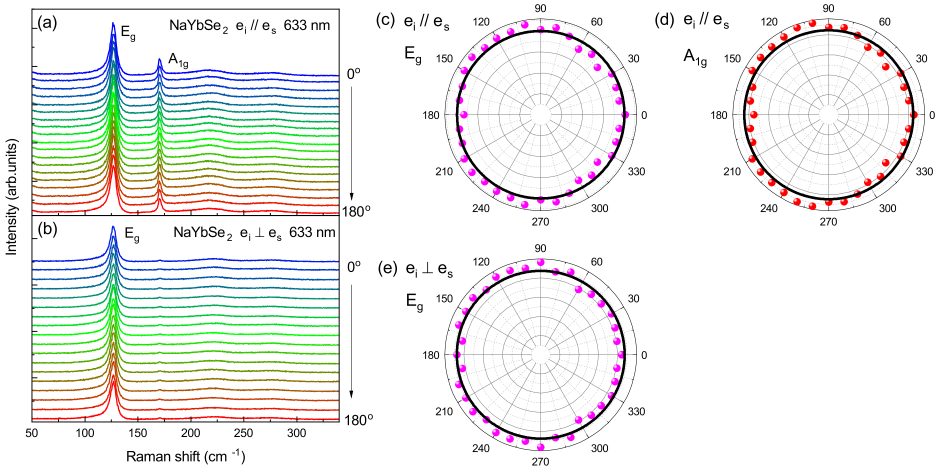


FIG. 7. $NaYbSe_2$ angle dependence raman experiments

$$E_{g,1} = \begin{pmatrix} c & 0 & 0 \\ 0 & -c & d \\ 0 & d & 0 \end{pmatrix} \tag{17}$$

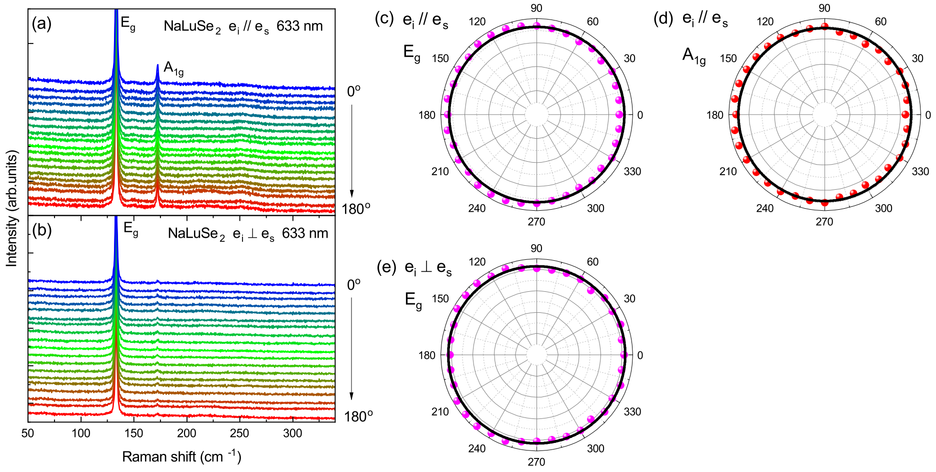


FIG. 8. $NaLuSe_2$ angle dependence raman experiments

$$E_{g,2} = \begin{pmatrix} 0 & -c & -d \\ -c & 0 & 0 \\ -d & 0 & 0 \end{pmatrix} \tag{18}$$

$$A_{1g} = \begin{pmatrix} a & 0 & 0 \\ 0 & a & 0 \\ 0 & 0 & b \end{pmatrix} \tag{19}$$

In parallel($e_i \parallel e_s$) and cross-polarization($e_i \perp e_s$) configurations, the scattering intensity of $E_g$ and $A_{1g}$ phonons changes with the rotation angle as follows:

$$E_g : I = c^2(e_i \parallel e_s) \tag{20}$$

$$A_{1g} : I = a^2(e_i \parallel e_s) \tag{21}$$

$$E_g : I = c^2(e_i \perp e_s) \tag{22}$$

$$A_{1g} : I = 0(e_i \perp e_s) \tag{23}$$

Where $I$ is the scattering intensity and $c$ and $a$ are constant. Because of the instrument, it is impossible to achieve complete extinction. Therefore, in FIG.7(a) and FIG.8(a), the phonon of $A_{1g}$ mode can also see a small amount of intensity in the cross-polarization configuration.

FIG. 7 and FIG. 8 show the $NaYbSe_2$ and $NaLuSe_2$ angle dependence raman experiments of $E_g$ and $A_{1g}$ phonons in different configurations respectively.

Based on the symmetry analysis, we also confirm that the vibration of the $E_g$ and $A_{1g}$ modes is from the Se atom in $NaYbSe_2$ and $NaLuSe_2$.

---


[1] T. Schleid and F. Lissner, Eur. J. Sol. Stat. Inorg. Chem. **30**, 829 (1993).

[2] M. Baenitz, P. Schlender, J. Sichelschmidt, Y. A. Onykiienko, Z. Zangeneh, K. M. Ranjith, R. Sarkar, L. Hozoi, H. C. Walker, J.-C. Orain, H. Yasuoka, J. van den Brink, H. H. Klauss, D. S. Inosov, and T. Doert, Phys. Rev. B **98**, 220409 (2018).

[3] W. Liu, Z. Zhang, J. Ji, Y. Liu, J. Li, X. Wang, H. Lei, G. Chen, and Q. Zhang, Chin. Phys. Lett. **35**, 117501 (2018).

[4] P. D. d. R. A. Bertin, Y. Chapuis and A. Yaouanc, J. Phys. Condens. Matter **24**, 256003 (2012).

[5] Y. Li, G. Chen, W. Tong, L. Pi, J. Liu, Z. Yang, X. Wang, and Q. Zhang, Phys. Rev. Lett. **115** (2015).

[6] D.J.Newman and B. Ng, *Crystal Field Handbook* (Cambridge University Press, 2000).

[7] I. Mirebeau, P. Bonville, and M. Hennion, Phys. Rev. B **76** (2007).

[8] M. Ruminy, E. Pomjakushina, K. Iida, K. Kamazawa, D. T. Adroja, U. Stuhr, and T. Fennell, Phys. Rev. B **94** (2016).

[9] E.Prince, *International Tables for Crystallography:Volume C* (Kluwer Academic Publisher, 2004).

[10] O. Arnold, J. Bilheux, J. Borreguero, A. Buts, S. Campbell, L. Chapon, M. Doucet, N. Draper, R. F. Leal, M. Gigg, V. Lynch, A. Markvardsen, D. Mikkelson, R. Mikkelson, R. Miller, K. Palmen, P. Parker, G. Passos, T. Perring, P. Peterson, S. Ren, M. Reuter, A. Savici, J. Taylor, R. Taylor, R. Tolchenov, W. Zhou, and J. Zikovsky, Nucl. Instrum. Methods. Phys. Res. A **764**, 156–166 (2014).

[11] M. Andrew, R. Applin, O. Arnold, A. Bamidele, L. Basso, J. Borreguero, E. Brown, H. Brown, N. Draper, M. Ganeva, M. A. Gigg, G. Guest, S. Hahn, S. Heybrock, A. J. Jackson, S. Jenkins, S. Jones, D. Le, R. Leal, A. Lim, J. Lin, V. Lynch, M. McDonnell, G. Miladinovic, L. Moore, D. Nixon, E. Oram, P. F. Peterson, V. Reimund, A. Russell, H. Saunders, A. Savici, A. Soininen, A. Sokolova, B. Sullivan, D. Tasev, T. Titcombe, R. Tolchenov, G. Vardanyan, R. Whitfield, and W. Zhou, "Mantid 4.1.0: Manipulation and analysis toolkit for instrument data," (2019).

[12] J. J. Baldoví, S. Cardona-Serra, J. M. Clemente-Juan, E. Coronado, A. Gaita-Ariño, and A. Palii, Journal of Computational Chemistry **34**, 1961–1967 (2013).

[13] H. Wondratschek and U. Muller, *International Tables for Crystallography:Volume A1* (Kluwer Academic Publisher, 2004).

[14] D. L. Rousseau, R. P. Bauman, and S. P. S. Porto, Journal of Raman Spectroscopy **10**, 253–290 (1981).
